# Supplementary material for: Stopping Criteria for Value Iteration on Stochastic Games with Quantitative Objectives
Source: arXiv:2304.09930 source file (2023-04-19)
Supplement: Supplementary file 1 [file 9_appendix_old.tex]

Puterman
212 Span norm [max V(s) - min V(s) for s in S]
365 Unichain/Multichain definition
381 VI for unichain
389: Prop 8.5.8: For any strat, the aperiodicity transformation "works"
390: Relative VI and action elimination might help in practice

[LL69] states that pure memoryless is enough. However, I'm not sure about rewards all being positive (in that paper).

Der hier macht das auch: Ehrenfeucht A, Mycielski J (1979) Positional strategies for mean-payoff games. Int J Game Theory 8:109–113

https://cs.au.dk/fileadmin/site_files/cs/PhD/PhD_Dissertations__pdf/koda_thesis.pdf#page=63 Super geiles Paper, das zeigt, dass alle wichtigen Spiele poly equiv sind; und vermutlich noch viel mehr praktisches. Außerdem zeigt es die Beziehung zwischen quantitative solving und strategically solving.

https://reader.elsevier.com/reader/sd/pii/S0304397517301391?token=C202E754E80787E4C20F5662D1D59C14500E77695F0B78815C479F35A210A4BBE747FA068D2D81BAAF9B89D34051DB4B&originRegion=eu-west-1&originCreation=20220105105422
Sollten wir erwähnen: Strat recovery for mean payoff is hard; but we have the TR value, not the MP value, so our problem is different.

need backup for the offset claim


Proof idea MP: Redo Zwick complexity of mean payoff games on graphs
Infinite game equiv to finite game equiv to limit of k step game.
Theorem 2.2: proof that limit of k step game is MP
[Instead of finding cycle, argue about agreeing on EC, i.e. in induced MC against optimal opponent strat, we have a BSCC.]


Finding value works by VI, as it is squeezed between k*V plusminus 2nW.

If an action is suboptimal for MP, it eventually is suboptimal for k-step TR, since convergence.
Thus, by picking actions optimal for k-step TR, eventually we pick optimal actions for MP.
Then we also ensure to reach a bottom MEC. There has to be one, and it has to be optimal. Previous ones might be optimal, too, but might also not be. [TR kinda should automatically force us to make progress, but I'm not sure about that.]

Additional argument: why don't we need memory? => Because we are safe and stopping.

For MP, also cite the pseudo-poly algos (I think there were more than just the one I have here. BWR games.)
https://link.springer.com/chapter/10.1007/978-3-642-39206-1_19 (conference)
https://www.sciencedirect.com/science/article/abs/pii/S0890540119300239 (journal)
https://link.springer.com/article/10.1007/s00453-017-0372-7 [Dunno, but some of the same people]
https://d1wqtxts1xzle7.cloudfront.net/43057047/pump-with-cover-page-v2.pdf?Expires=1641392186&Signature=NX8Jqhvn~rIgiN53Mw7FoIq9jXuAI4eV5WA-XShoVgbxi4fc7-pIGz2bVbXcxr2MJPFx2EAPHOCsPOwemjL4dQTMszT9vOaGN0FFDk54LKLaa512t2zHZ~60bDqlwK5FRIdlp-WIYx2cMm9UAbJdmxBrDLV9wcCQpKaqtxrDExwimY-9Xw228QvWBrEo0jK4oOdFQYyYiP~cCwRU0vk4B1U7cGkaAYRlS0Ene82MvYSLuxLOdU-Oh8deoPVzFhBW5mH9IgnKxyO~LMJcxBgNEy5~XFsg7TQOLxZjFcSv7prThpwIqlUEaYBzb8cmQl2nK9ZUaqqdYH06tCbnuFA-YA__&Key-Pair-Id=APKAJLOHF5GGSLRBV4ZA [This one only for ergodic]
Also talking about ergodic: https://link.springer.com/chapter/10.1007/978-3-662-43951-7_11
We can say that for SMPG, there were some attempts, but nothing really good except for the proof that it can be reduced and the conjecture that it should be easy.


\section{Obtaining Strategies from Values (Lemma \ref{lem:VIrecommend})} \label{app:strategies_from_values}
%
In this appendix, we explain how\footnote{The following description is partly taken from the journal version of \cite{KKKW18}, which is currently under submission. We put it here for readers convenience and will include the proper reference as soon as possible.}, given a sequence of value-vectors as computed by value iteration, one can obtain a strategy that achieves at least that value.
This suffices to prove Lemma \ref{lem:VIrecommend}, since classical value iteration computes monotonic convergent sequence of values vectors (see~\cite{DBLP:conf/spin/ChatterjeeH08} for reachability and safety, ~\cite{SGreward} for total rewards and Appendix \ref{app:mean_payoff} for mean payoff), and thus the recommended strategies eventually are optimal.

\input{9a_strats}

%
%
%We first briefly outline the well-known approach to obtain strategies from the finite prefix objectives we consider.
%For reachability, safety, and total reward, observe that the values $v_i$ obtained in value iteration always correspond exactly to the optimal $i$-step value, i.e.\ \enquote{what is the optimal probability of reaching the target within $i$ steps} and analogous for safety and total reward.
%Moreover, it is well known that given a state $s$ choosing $\argopt_{a \in \act(s)} \sum_{s' \in \allstates} \trans(s, a, s') \cdot v_{i-1}(s')$ yields an optimal choice for these $i$-step properties.\footnote{Of course, at step $i - 1$ we need to choose optimally using $v_{i-2}$ etc.}
%Formally, if $\Phi_i$ is such an $i$-step objective, we have for all $s$ that $\val_{\G, \Phi_i}(s) = v_i(s)$.
%An action $a$ chosen w.r.t.\ the above equation thus optimizes the expected value obtainable in $i - 1$ steps and $a$ is an optimal choice in state $s$ for an $i$-step objective.
%Next, observe that the finite horizon variants of the three considered objectives are monotone w.r.t.\ the horizon.
%Formally, we have $\val_{\G, \Phi_i} \leq \val_{\G, \Phi_{i + 1}} \leq \val_{\G, \Phi}$ (or $\geq$ in the case of safety) and analogous for a fixed strategy.
%Intuitively, in the case of, e.g.\ reachability, having more time to reach the target never hurts.
%Now, define $\straa_i$ as the strategy that chooses such an $i$-step optimal action $a$ in every state.
%Combining the above observations, we see that if we employ $\straa_i$ in the infinite horizon setting it achieves at least (or, in the case of safety, at most) a value of $\val^{\straa_i, \cdot}_{\G, \Phi} \geq \val^{\straa_i, \cdot}_{\G, \Phi_i} = v_i$.
%
%Moreover, recall that $v_i$ is monotonically improving and converges to the true value in the limit.
%Additionally, there are only finitely many memoryless deterministic strategies, hence eventually the obtained strategy has to be an optimal one:
%Assume that $\straa_i$ is optimal for the infinite horizon.
%Since $v_i$ can only improve, we also have that $\straa_j$ is optimal for all $j > i$.
%Note that potentially $\straa_i \neq \straa_j$, however this still satisfies our assumptions.
%
\section{Additional Proofs for Mean Payoff}\label{app:mean_payoff}
%
\subsection{Convergence of Value Iteration} \label{app:mean_payoff:vi_convergence}
%
In this section, we prove that (i)~when $v_i$ is iterated according to Equation~\eqref{eq:bellmanTR}, we have that $v_i / i$ converges to the true value and (ii)~by following $v_i$, we eventually obtain optimal strategies.
%
%By \cite{liggett1969stochastic,DBLP:conf/isaac/AnderssonM09} (see also \cite{DBLP:journals/ejcon/SvorenovaK16}) we have that for every game and mean payoff objective, there exists a threshold $\beta_1$ such that for all discount factors $\beta_1 \leq \beta < 1$, we have that any strategy optimal for the $\beta$-discounted total reward, i.e.\ $\Phi(\infinitepath) = \sum_{i=0}^\infty \beta^i \cdot \reward(\infinitepath_i)$, is also optimal for the mean payoff.
%Similarly, we have that there exists a threshold $\beta_2$ such that for all discount factors $\beta_2 < \beta < 1$, we have that any strategy optimal for total reward is also optimal for $\beta$-discounted total reward.
%Observe that following $v_n$ eventually yields strategies optimal for the total expected reward as argued above.
%By choosing $\beta$ appropriately, we have that this strategy is $\beta$-discounted reward optimal and in turn also mean payoff optimal.
%
%
%
Here, we cannot follow the same line of reasoning as before, since we actually iterate the $n$-step total reward.
However, we can transfer existing proofs to the world of stochastic games.
In particular, the (quite lengthy) reasoning of \cite[Sec.~9]{DBLP:books/wi/Puterman94} (culminating in Thm.~9.4.5), which proves similar statements for mean payoff value iteration on MDP, mainly uses the induced Markov chain and its transition matrix.
As such, the proofs for games work analogous in most places.
We provide the major definitions and claims here and point the interested reader at the respective sections.
Moreover, we supply relevant, related theorems from the literature.

We begin by introducing the \emph{mean payoff optimality equations} \cite[Sec.~9.1.1]{DBLP:books/wi/Puterman94}.
For every state $s$, they require that
\begin{align*}
	g(s) & = \opt_{a \in \act(s)} {\sum}_{s' \in \allstates} \trans(s, a, s') \cdot g(s'), \text{ and} \\
	h(s) & = \reward(s) - g(s) + \opt_{a \in \act_g(s)} {\sum}_{s' \in \allstates} \trans(s, a, s') \cdot h(s'),
\end{align*}
where $\act_g(s) \eqdef \{a \in \act(s) \mid g(s) = {\sum}_{s' \in \allstates} \trans(s, a, s') g(s')\}$, i.e.\ the witnesses for the first line.
Here, $g$ is called \emph{gain} and $h$ is called \emph{bias}.
Intuitively, the gain equals the value of the mean payoff game while the bias describes how much total expected deviation from the gain is obtained starting from some state.
For example, consider the sequence of values $10\ 12\ 5\ 5\ 5\ \cdots$.
Here, we have that the mean payoff would equal $5$ while the bias would equal $5 + 7 + 0 + 0 + \cdots = 12$.
%Observe that the system of equations is \enquote{nested}, since $g$ and $\act_g$ occur in the optimality equation of $h$.

On MDP, the gain part of any solution to these equations equals the value of the game (see \cite[Sec.~9.1.2,~9.1.3]{DBLP:books/wi/Puterman94}) and these optimality equations give a characterization of optimal strategies \cite[Sec.~9.1.4]{DBLP:books/wi/Puterman94}.
Now, given that memoryless deterministic strategies are optimal for mean payoff \cite{liggett1969stochastic,bewley1978stochastic}, we can extend this reasoning to games by applying it to both induced MDP.\footnote{To directly replicate the proof structure of \cite{DBLP:books/wi/Puterman94}, observe that (i)~memoryless deterministic strategies are optimal for discounted reward games due to \cite{shapley} or \cite{DBLP:journals/mmor/RaghavanF91} and (ii)~for a large enough discount factor, we have that discount-optimal strategies are also mean payoff optimal \cite{liggett1969stochastic}.}
An abstract proof of the properties of these optimality equations, presented in a rather different formalism, can be found in \cite{DBLP:conf/cdc/AkianCDG13} (see especially Eq.~(5)).

To prove convergence of VI \cite[Sec.~9.4]{DBLP:books/wi/Puterman94}, fix $g^\ast, h^\ast$ a solution to the optimality equations and let $(\straa^\ast, \strab^\ast)$ be a pair of optimal strategies.
It remains to show that the limit of
\begin{equation*}
	e_i(s) = v_i(s) - i \cdot g^\ast(s) - h^\ast(s)
\end{equation*}
exists.
Then, we have that both $v_{i+1} - v_i$ and $v_i / i$ converges to $g^\ast$ and the strategies following $v_i$ eventually are optimal (using the fact that only finitely many memoryless deterministic strategies exist).
The proofs of \cite{DBLP:books/wi/Puterman94} go through without significant modification.
For most proofs, it is sufficient to replace the optimal witness $\delta$ strategy with the joint strategy $\pi^\ast(s) = \straa^\ast(s)$ for $s \in \maxstates$ and $\strab^\ast(s)$ otherwise.
One major requirement used in Thm.~9.4.4 and 9.4.5 is the notion of \emph{aperiodicity}.
Essentially, this requires that for any pair of fixed strategies, the induced Markov chain is aperiodic, i.e.\ for a pair of states $s$ and $s'$ we either have that there exists no path from $s$ to $s'$ or we have that the probability of reaching $s'$ after exactly $n$ steps starting from $s$ in the chain is non-zero for any $n \geq |\allstates|$.
Technically, this ensures that the steady state transition matrix $P^* = \lim_{n \to \infty} P^n$ of the induced Markov chain exists.
Fortunately, this assumption can be ensured by an \emph{aperiodicity transformation} \cite[Sec.~8.5.4]{DBLP:books/wi/Puterman94}, which essentially modifies every action to include a small loop back to the originating state.
It also is straightforward to see that this preserves optimal strategies and only changes the value of the game by a known multiplicative constant \cite[Cor.~8.5.9]{DBLP:books/wi/Puterman94}.

In total, we obtain that (i)~$\lim_{i \to \infty} v_i / i = \lim_{i \to \infty} v_{i+1} - v_i = \val_{\G, \Phi}$ for mean payoff objectives and (ii)~choosing an optimal action w.r.t.\ $v_i$ eventually yields an optimal strategy.
%Note that in the case of multiple optimal strategies, it can happen that the recommender alternates between them.
%
\subsection{Bounds for Mean Payoff} \label{app:mean_payoff:span_norm}
%
As with the other objectives, the iteration for mean payoff does not give us a \emph{stopping criterion}, i.e.\ we do not know how close we are to the true solution.
However, under some assumptions, we can indeed use the iterates themselves to derive both upper and lower bounds.
In the MDP world, \cite[Sec.~8.5]{DBLP:books/wi/Puterman94} suggests to inspect the difference vector $\Delta_i \eqdef x_{i+1} - x_i$, i.e.\ the reward gained in the $i+1$-th step.
Assuming that all states of an MDP have the same optimal value $v$, one can show that
\begin{equation}
	\min_{s \in \allstates} \Delta_i(s) \leq v \leq \max_{s \in \allstates} \Delta_i(s). \label{eq:mean_payoff_span_equation}
\end{equation}
In \cite{DBLP:conf/cav/AshokCDKM17}, the authors show how to utilize this property for the general case.
The central observation is that once we restrict ourselves to a MEC, all states necessarily have the same value.
Thus, in a nutshell, by restricting to a MEC and running value iteration until convergence, we obtain the optimal value the system can achieve (assuming it decides to stay inside this MEC).
Once these values are computed for each MEC, \cite{DBLP:conf/cav/AshokCDKM17} proposes to propagate them through the complete MDP via a variant of reachability.

In our application, we can analogously use this insight to derive bounds on the staying values of ECs in the induced MDPs.
Naively, whenever we want to determine the staying value of a MEC, we can simply run a value iteration in the restricted MDP akin to \cite{DBLP:conf/cav/AshokCDKM17} until convergence.
However, we can use additional insights for a more sophisticated approach.
Firstly, instead of starting from scratch, we can use the current value vector $v_i$ as starting vector for the iteration in each MEC, since Equation~\eqref{eq:mean_payoff_span_equation} holds for any starting value.
Note that the delta vector obtained from these $v_i$ may not necessarily be close to the staying value, as the value of a state may be much higher (or lower) than the staying value.
Observe that in Algorithm~\ref{alg:SG-view}, staying values are important to decide whether the current player prefers to remain inside the EC or (try to) leave it.
If after some steps of iteration, it turns out that the upper bound obtained through Equation~\eqref{eq:mean_payoff_span_equation} is smaller than the identified best Maximizer exit, we can immediately stop the iteration:
It is clear that Maximizer prefers the best exit and $\mathcal{U}$ will take that value.
Dually, if the obtained lower bound on the staying value is larger than the best exit value, we know that (given the strategy of the opponent) the current player prefers to stay and we do not need to deflate.
Of course, both of arguments dually apply to the lower bounds and inflating.
Finally, instead of computing the upper bound overly precise each time, we can successively tighten the required precision of the staying value approximation (related to the on-demand approach of \cite{DBLP:conf/cav/AshokCDKM17}).


\section{Upper Bound Initialization}\label{app:u-init}

Here we define the upper bound initialization $\text{Upper\_VI\_Value}_\Phi$ as it is used in Algorithm~\ref{alg:SG-view}.
For reachability and safety, 1 is a correct upper bound, as that is the highest possible value. For mean payoff, $\max_{s \in \allstates} \reward(s)$ is the highest possible value.
The only more involved case is total reward:
For correctness, it is necessary to set the upper bound to $\infty$ for all states that can achieve infinite reward.
We detect those in the usual ways, see~\cite{SGreward}.
For the remaining states, we must not use $\infty$, as otherwise the Bellman update cannot converge.
We instead compute a rational number that is greater than the highest possible non-infinite total reward, using a straightforward extension of the procedure from~\cite[Sec.~3.3]{ensuring} to SGs.
In essence, the idea is as follows:
Let $p_{\min}$ denote the minimum transition probability in the SG and let $s$ be any state with non-infinite value.
Fix optimal strategies $(\straa^\ast, \strab^\ast)$.
Since $s$ has a finite value, the probability to eventually reach a target state or a region where zero rewards are obtained equals one in $\G^{\straa^\ast, \strab^\ast}$.
From classical observations on Markov chains \cite{DBLP:books/daglib/0020348}, we thus know that there is a probability of at least $p_{\min}^{\abs{\allstates}}$ for this to happen within $\abs{\allstates}$ steps (the smallest possible probability of a path of length $n$).
This path can obtain at most $R_{\max} = \abs{\allstates} \cdot \max_{s \in \allstates} \reward(s)$ reward.
Hence, the maximum total reward can be bounded by $\sum_{i = 1}^\infty (1 - p_{\min}^{\abs{\allstates}})^i R_{\max}$.
In \cite[Sec.~3.3]{ensuring}, there are more refined ways of approximating.

%\clearpage % Keep this the last Appendix
%\section{Abstract Variant of Algorithm~\ref{alg:MDP-view}}\label{app:abstractAlgo}
%\begin{algorithm}[!h]
%	\caption{Generic anytime algorithm based on global reduction to MDP} \label{alg:abstract}
%	\begin{algorithmic}[1]
%		\Require SG $\G$, Objective $\Phi$, initial state $\initstate$, and precision $\varepsilon$
%		\Ensure $(\lb, \ub)$ such that $\lb \leq \val \leq \ub$ and $\ub(\initstate) - \lb(\initstate) \leq \varepsilon$
%		\Commentline{Initialization}
%		\State Initialize the recommender procedure
%		\State $\lb_0(\cdot) \gets 0$ \Comment{Lower and \hspace*{8.5mm}~}
%		\State $\ub_0(\cdot) \gets +\infty$ \Comment{upper bounds\hspace*{5.5mm}~}
%		\State $i \gets 0$
%		\Repeat
%		\Statex \Commentline{Recommender procedure}
%		\State Perform an iteration of the recommender procedure
%		\State $\straa, \strab \gets$ strategies from the recommender procedure
%		\medskip
%		\Statex \Commentline{Compute bounds}
%		\State $\lb_{i+1} \gets \max(\lb_i, \val(\G^{\straa,\cdot})) $
%		\State $\ub_{i+1} \gets \min(\ub_i, \val(\G^{\cdot,\strab})) $
%		\medskip
%		\State $i \gets i + 1$
%		\Until{$\ub_i(\initstate)-\lb_i(\initstate) \leq \varepsilon$}
%	\end{algorithmic}
%\end{algorithm}

\section{Strategy Iteration Variant of Algorithm~\ref{alg:MDP-view}}\label{app:SIversion}
\begin{algorithm}[!h]
	\caption{Generic strategy iteration anytime algorithm} \label{alg:abstract}
	\begin{algorithmic}[1]
		\Require SG $\G$, Objective $\Phi$, initial state $\initstate$, and precision $\varepsilon$
		\Ensure $(\lb, \ub)$ such that $\lb \leq \val \leq \ub$ and $\ub(\initstate) - \lb(\initstate) \leq \varepsilon$
		\Commentline{Initialization}
		\State Initialize the recommender procedure
		\State $\lb_0(\cdot) \gets 0$ \Comment{Lower and \hspace*{8.5mm}~}
		\State $\ub_0(\cdot) \gets \infty$ \Comment{upper bounds\hspace*{5.5mm}~}
		\State $\straa \gets$ arbitrary Maximizer strategy
		%\State $\strab \gets$ arbitrary Minimizer strategy
		\State $i \gets 0$
		\Repeat
		\State $i \gets i + 1$
		\medskip
		\Statex \Commentline{Recommender procedure}
		\State $x \gets \val(\G^{\straa,\cdot})$\label{line:si-mdp}
		\State $\straa, \strab \gets$ best-effort strategies inferred from $x$
		\medskip
		\Statex \Commentline{Compute bounds}
		\State $\lb_{i} \gets x $
		\State $\ub_{i} \gets \val(\G^{\cdot,\strab}) $\label{line:si-u}
		\Until{$\ub_i(\initstate)-\lb_i(\initstate) \leq \varepsilon$}
	\end{algorithmic}
\end{algorithm}

Note that, in a sense, $\strab$ is already computed implicitly in Line~\ref{line:si-mdp} when solving the MDP, because solving the MDP requires computing the optimal counter-strategy to $\straa$.
So when obtaining $\straa$ and $\strab$ from $x$, $\strab$ is exactly the globally optimal strategy in the MDP $\G^{\straa,\cdot}$; in contrast, the new Maximizer strategy $\straa$ is only locally optimal against $\strab$.
Trying to use a global best response to $\strab$, i.e. solving the MDP $\G^{\cdot,\strab}$, can result in cyclic behaviour and non-convergence to the optimal strategies~\cite{condonAlgo}.
This is why the computation of $\ub_i$ does not affect the choice of the next strategies at all, but only serves to provide an upper bound.
This is also the only real difference to classic strategy iteration: the additional computation of the upper bound in Line~\ref{line:si-u}.
